# Supplementary material for: Finite-temperature criticality through quantum annealing
Source: arXiv:2507.07167 ancillary file (2025-07-09)
Supplement: Supplementary file 1 [file SM.pdf]

# Supplemental Material for :"Finite temperature criticality through quantum annealing"

Gianluca Teza,[1, a)] Francesco Campaioli,[2, 3, b)] Marco Avesani,[4, 5, c)] and Oren Raz[6, d)]

[1)] *Max Planck Institute for the Physics of Complex Systems, Nöthnitzer Str. 38, 01187 Dresden, Germany*

[2)] *Department of Physics, School of Science, RMIT University, Melbourne, Victoria, Australia*

[3)] *Dipartimento di Fisica e Astronomia G. Galilei, Universitá degli Studi di Padova, 35131 Padova, Italy*

[4)] *Dipartimento di Ingegneria dell'Informazione, Universitá degli Studi di Padova, 35131 Padova, Italy*

[5)] *Padua Quantum Technologies Research Center, Università degli Studi di Padova, via Gradenigo 6B, IT-35131 Padova, Italy*

[6)] *Department of physics of complex systems, Weizmann institute of science, Rehovot, Israel, 76100*

(Dated: 9 July 2025)

In this supplemental material (SM) we discuss the details of the calculations and results presented in the main text.

## I. DERIVATION OF THE QUANTUM NUCLEATION BARRIER IN THE 2D TRANSVERSE-FIELD ISING MODEL

This section provides the derivation and physical justification for the expression used to estimate the nucleation barrier between metastable and stable states in the two-dimensional transverse-field Ising model (TFIM) at zero temperature (Eq. in the main text). The formula used in the main text is rooted in a semi-classical extension of classical nucleation theory via a Suzuki-Trotter mapping of the quantum model to an effective (2+1)-dimensional classical model[?] .

### A. Physical Model

We consider the TFIM Hamiltonian with a small longitudinal field:

$$\hat{H} = -J\left(\sum_{\langle ij\rangle} \hat{\sigma}_i^z \hat{\sigma}_j^z + \epsilon \sum_i \hat{\sigma}_i^z\right) - \Gamma \sum_i \hat{\sigma}_i^x,$$

where:

- $J > 0$ is the ferromagnetic coupling,
- $\Gamma$ is the transverse field introducing quantum fluctuations,
- $\epsilon \ll 1$ is a small longitudinal bias field selecting one magnetization sector.

For the following estimation, the system is taken at zero temperature ($T = 0$) with $\Gamma < \Gamma_c$, where $\Gamma_c \approx 3.04J$ marks the quantum critical point beyond which long-range order disappears[? ?] .

### B. Suzuki–Trotter Mapping

To analyze quantum nucleation in the 2D TFIM, we use the Suzuki–Trotter decomposition to map the quantum model at inverse temperature $\beta$ to a classical Ising model in (2+1) dimensions. In this mapping, the original two

[a)] Electronic mail: teza@pks.mpg.de
[b)] Electronic mail: francesco.campaioli@unipd.it
[c)] Electronic mail: marco.avesani@dei.unipd.it
[d)] Electronic mail: oren.raz@weizmann.ac.il

spatial dimensions remain intact, while the imaginary-time dimension is discretized into $M = \beta/\Delta\gamma$ slices, where $\Delta\gamma$ is the Trotter time step. The resulting classical model is defined on a cubic lattice of size $L \times L \times M$, with anisotropic nearest-neighbor couplings:

$$K = J\Delta\gamma, \quad K_\gamma = -\frac{1}{2}\log\tanh(\Gamma\Delta\gamma),$$

corresponding to the spatial and temporal directions, respectively.

The longitudinal field $J\epsilon$ in the quantum model becomes an effective field $J\epsilon\Delta\gamma$ per time slice in the classical model. In this framework, quantum tunneling processes are interpreted as thermally activated droplet formation in Euclidean spacetime.

### C. Calibrating the Model

Although the Suzuki–Trotter mapping becomes exact in the limit $\Delta\gamma \to 0$, we adopt a finite value of $\Delta\gamma$ for practical and conceptual convenience. Since we work in the zero-temperature limit $T \to 0$, the number of Trotter slices $M = \beta/\Delta\gamma$ diverges even at fixed $\Delta\gamma$, ensuring convergence of the mapping.

To calibrate $\Delta\gamma$, we use the fact that the mapped (2+1)-dimensional classical Ising model becomes critical when its spatial coupling equals the known critical coupling of the 3D classical Ising model:

$$K = J\Delta\gamma = K_c^{(3D)} \approx 0.2216.$$

Solving for $\Delta\gamma$, we find:

$$\Delta\gamma = \frac{K_c^{(3D)}}{J}.$$

Using the experimental value $J \approx 0.3212\,\text{GHz}$, this gives:

$$\Delta\gamma \approx \frac{0.2216}{0.3212} \approx 0.69\,\text{ns}.$$

This calibrated time step ensures that the spatial coupling in the mapped 3D model reaches the classical critical point when the 2D TFIM reaches its known quantum critical value $\Gamma_c \approx 3.04J$. The temporal coupling at this point is then:

$$K_\gamma(\Gamma_c, \Delta\gamma) = -\frac{1}{2}\log\tanh(\Gamma_c\Delta\gamma),$$

which can be verified to also approach $K_c^{(3D)}$, confirming consistency of the mapping.

### D. Semi-Classical Droplet Action

We analyze the nucleation of a droplet of the stable phase (aligned with $h$) within a metastable background. Near $T = 0$, such nucleation occurs via quantum tunneling, modeled as the formation of a compact droplet in 3D Euclidean space-time.

The action cost $\Delta\mathcal{S}(R, \ell)$ for a cylindrical droplet of spatial radius $R$ and temporal extent $\ell$ is:

$$\Delta\mathcal{S}(R, \ell) = 2\pi R\ell \cdot \sigma + \pi R^2 \cdot \sigma_\gamma - \pi R^2 \ell \cdot \Delta f,$$

where:

- $\sigma$ is the spatial domain wall tension, i.e., the energy cost per unit length of domain wall in space. At $\Gamma = 0$, it takes the classical value $\sigma_0 = 2J$ in lattice units. For $\Gamma > 0$, quantum fluctuations soften domain walls, and we model this as $\sigma(\Gamma) = \sigma_0\,(1 - \Gamma/\Gamma_c)^\mu$.
- $\sigma_\gamma$ is the temporal wall tension, representing the action cost per unit area of the droplet caps in imaginary time. It arises from the transverse field $\Gamma$, and is given by $\sigma_\gamma(\Gamma) = -\frac{1}{2}\log\tanh(\Gamma\Delta\gamma)$. As expected, it vanishes at $\Gamma = 0$, where no tunneling occurs.
- $\Delta f = 2m(\Gamma)J\epsilon$ is the energy density difference due to the longitudinal field,

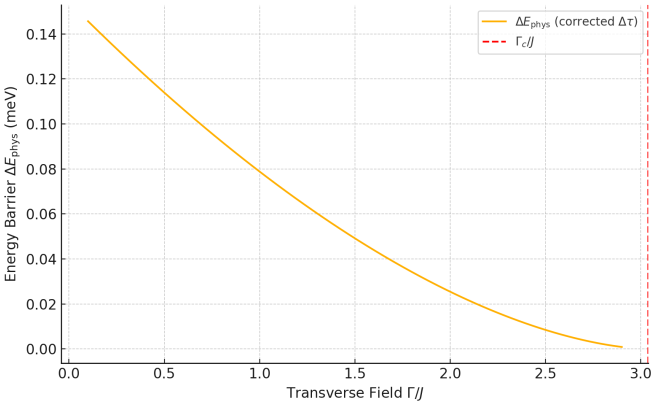


FIG. 1. Barrier height as a function of $\Gamma$, estimated using nucleation theory for $\epsilon = 0.05$ and $J \approx 0.3212\,\text{GHz}$.

- $m(\Gamma)$ is the spontaneous magnetization at transverse field $\Gamma$.

Extremizing this action with respect to $R$ and $\ell$ yields the saddle-point droplet configuration, which determines the dominant contribution to the tunneling action: Extremizing this action with respect to $R$ and $\ell$ gives the critical droplet configuration that dominates the tunneling process. The partial derivatives are:

$$\frac{\partial \Delta \mathcal{S}}{\partial \ell} = 2\pi R \cdot \sigma - \pi R^2 \cdot \Delta f = 0 \quad \Rightarrow \quad R_c = \frac{2\sigma}{\Delta f},$$

$$\frac{\partial \Delta \mathcal{S}}{\partial R} = 2\pi \ell \cdot \sigma + 2\pi R \cdot \sigma_\gamma - 2\pi R \ell \cdot \Delta f = 0 \quad \Rightarrow \quad \ell_c = \frac{\sigma_\gamma}{\Delta f}.$$

The physical energy barrier is then given by the dimensionful expression:

$$\Delta E_{\rm phys}(\Gamma, \epsilon) = \frac{\hbar \Delta \mathcal{S}_c}{\ell_c \Delta\gamma} = \frac{2\pi\hbar\sigma^2(\Gamma)}{\Delta\gamma \cdot m(\Gamma) J \epsilon}.$$

We model the dependencies of $\sigma$ and $m$ on the transverse field using scaling forms:

$$\sigma(\Gamma) = \sigma_0 \left(1 - \frac{\Gamma}{\Gamma_c}\right)^{\mu}, \quad m(\Gamma) = \left(1 - \frac{\Gamma}{\Gamma_c}\right)^{\beta},$$

where $\sigma_0 = 2J$, $\mu \approx 1$ (see[?] ), and $\beta \approx 0.32$ (see[?] ). Substituting the empirical scaling forms and using $\sigma_0 = 2J$, we obtain:

$$\Delta E_{\rm phys}(\Gamma, \epsilon) = \frac{2\pi\hbar(2J)^2}{\Delta\gamma \cdot J\epsilon} \cdot \left(1 - \frac{\Gamma}{\Gamma_c}\right)^{2\mu-\beta} = \frac{8\pi\hbar J}{\Delta\gamma \cdot \epsilon} \cdot \left(1 - \frac{\Gamma}{\Gamma_c}\right)^{2\mu-\beta} = \frac{8\pi\hbar J^2}{K_c^{(3D)}\epsilon} \cdot \left(1 - \frac{\Gamma}{\Gamma_c}\right)^{2\mu-\beta}.$$

All quantities in this expression are in physical units, and $\Delta E_{\rm phys}$ has units of energy.

In the relevant experimental conditions in the main text, we used $\epsilon = 0.05$ and $J \approx 0.3212\,\text{GHz}$. For these values, $\Delta E_{phys}(\Gamma)$ is plotted in Fig. 1.

M. Suzuki, Progress of theoretical physics **56**, 1454 (1976).
Z. Friedman, Phys. Rev. B **17**, 1429 (1978).
S. Hesselmann and S. Wessel, Phys. Rev. B **93**, 155157 (2016).
M. Hasenbusch and K. Pinn, Physica A: Statistical Mechanics and its Applications **192**, 342 (1993).
A. Talapov and H. Blöte, Journal of Physics A: Mathematical and General **29**, 5727 (1996).
